# Supplementary material for: Investigating the Limits of Hard X-ray Coherence Length Measurement Employing Young's Double Slit Experiment
Source: arXiv:2410.13172 source file (2025-03-26)
Supplement: Supplementary file 1 [file Suppli_Investigating_Limits_of_Coherence_Length_Measurements.pdf]

# Supplemental Information

March 18, 2025

## S1 Detector Details

Horizontal coherence length measurements were taken using a mono beam microscope from optiquepeter with a PCO 4000 camera using a 4× magnification setting. The physical pixel size of the PCO 4000 camera is $9 \times 9$ µm. Vertical coherence length measurements were taken with a mono beam microscope from optiquepeter with a PCD Edge 4.2 bi camera using a 9× magnification setting. The physical pixel size of this camera is $6.5 \times 6.5$ µm. Effective pixel sizes for the vertical and horizontal measurements have been determined to be 0.7 µm and 3.1 µm, respectively. Effective pixel sizes were directly measured from the images taken during the experiment through interference fringe width through the procedure outlined in Section S5.

## S2 SEM Imaging of Double Slits

SEM images were taken of the various double slits to verify the slit parameters. In some cases, asymmetry was observed in the recorded interference patterns. Additionally, a small affine transformation was present in the numerically fitted interference fringes before using the correct slit parameters during the fitting procedure. Fig. S1 to Fig. S4 display the SEM images taken of the double slits. Table 1 displays the slit parameters that were measured from the images.

## S3 Vertical Coherence Length Measurements

The results of 2 vertical component measurements is shown in Fig. S6. Values range from 24.9 µm to 51.2 µm which are 3 times compared to what was observed in the horizontal component. The energy used for the vertical spatial coherence length measurement was 6.85 keV.

## S4 Asymmetry in the Observed Interference Patterns

In this supplemental section, we provide simulated double slit interference patterns to demonstrate that the asymmetry observed in our experiment can be attributed to one of the slits being wider than the other. For the simulation, the diffractio python library has been used. More detailed information about this library can be found here https://diffractio.readthedocs.io.To begin, a plane wave source of $E = 9.6$ keV has been defined. This corresponds to the energy at which the asymmetry started to become more noticeable. Two masks are then constructed for

this simulation. The first is for an ideal double slit with slit widths of 3 µm and a slit separation of 10 µm, identical to the double slit we observed to have one slit wider than the other. The second mask is a single slit with a width of 1um. The two masks are summed such that the center of the single slit is added to the edge of one of the double slits, which will result in an asymmetric double slit as shown in Fig. S7. The wave propagation after the slit is then observed by placing the "detector" 6 m from the double slit, as performed in the experiment. Using the ideal double slit where both slits have the same width, we observe the expected symmetric intensity distribution. However, while including the asymmetric slit widths, a skewed intensity distribution is observed. Though the simulation did not include the exact slit dimensions recorded by SEM measurements, the 1 $\mu$m slit width asymmetry is included in the simulation, and a skewed fringe pattern is still observed. The simulated symmetric and asymmetric fringes are shown in Fig. S8 and S9.

# S5 Effective Pixel Size Calculation

In this supplemental section, we provide a sample calculation to determine the effective pixel size directly from images obtained from the PCO detector, as well as report the effective pixel sizes obtained from the rest of the images. The effective pixel sizes are found using the interferomic fringe width which is defined to be

$$w = \frac{\lambda L}{d}. \tag{1}$$

Using the same definitions as before, $\lambda$ represents the X-ray wavelength, $L$ represents the sample-to-detector distance, and $d$ is the slit separation. The result can be found in many standard optics texts. For this sample calculation, we will use the image `Image156.tif` from our data set, where $E$ = 6.75 keV ($\lambda$=1.837$\mathring{A}$), $L$ = 6 m, and $a$ = 11.612 µm. From this, we determine that the fringe with for this X-ray energy and double slit separation is

$$w = \frac{(1.837 \times 10^{-10}\text{m})(6\text{m})}{11.612 \times 10^{-6}\text{m}} = 94.921\mu\text{m}$$

As shown in Fig. S10, the fringe width from the image is 28 pixels. This provides an effective pixel size of 3.39 µm. Using this same procedure, the effective pixel sizes from the rest of the images collected from this experiment are reported in Table 2. The average pixel sizes determined through this procedure are $2.984 \pm 0.149$µm for the horizontal measurements, and $0.752 \pm 0.043$µm for the vertical measurement.

| Double slit | Slit 1 Measurement (µm) | Slit 2 Measurement (µm) | Slit separation Measurement ($\mu$m) |
|---|---|---|---|
| 10 µm | $3.265 \pm 0.021$ | $2.585 \pm 0.019$ | $11.612 \pm 0.020$ |
| 20 µm | $3.240 \pm 0.009$ | $3.248 \pm 0.011$ | $20.909 \pm 0.019$ |
| 50 µm | $3.841 \pm 0.013$ | $4.004 \pm 0.014$ | $51.685 \pm 0.015$ |
| 100 µm | $3.981 \pm 0.014$ | $3.977 \pm 0.008$ | $100.770 \pm 0.021$ |

Table 1: Displayed are the physical measurements taken of each double slit using the SEM images obtained.

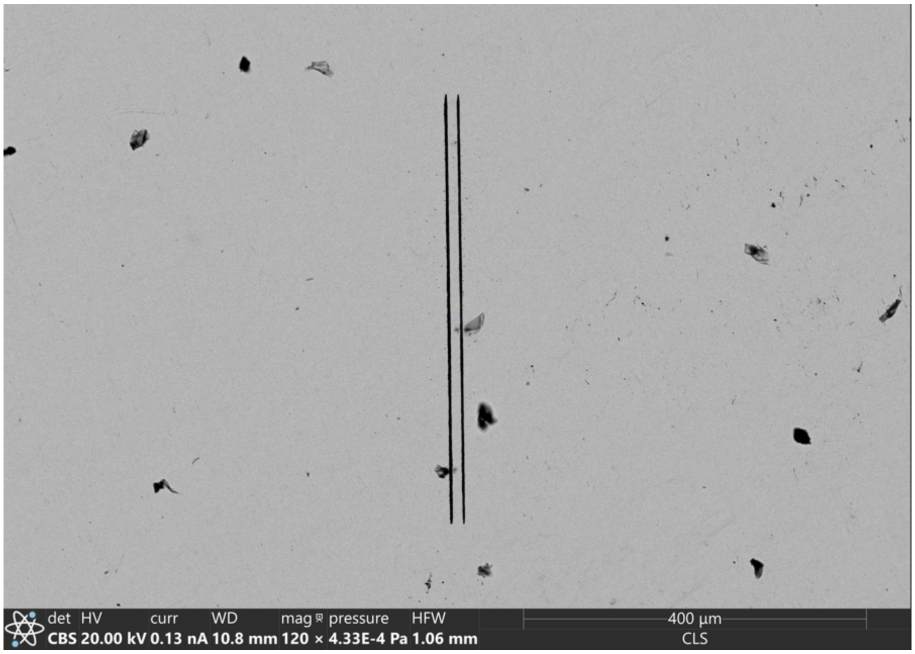


Fig. S1: Displayed is the SEM image taken for the 10 µm double slit. It is apparent in the image that the right slit is thinner than the left slit.

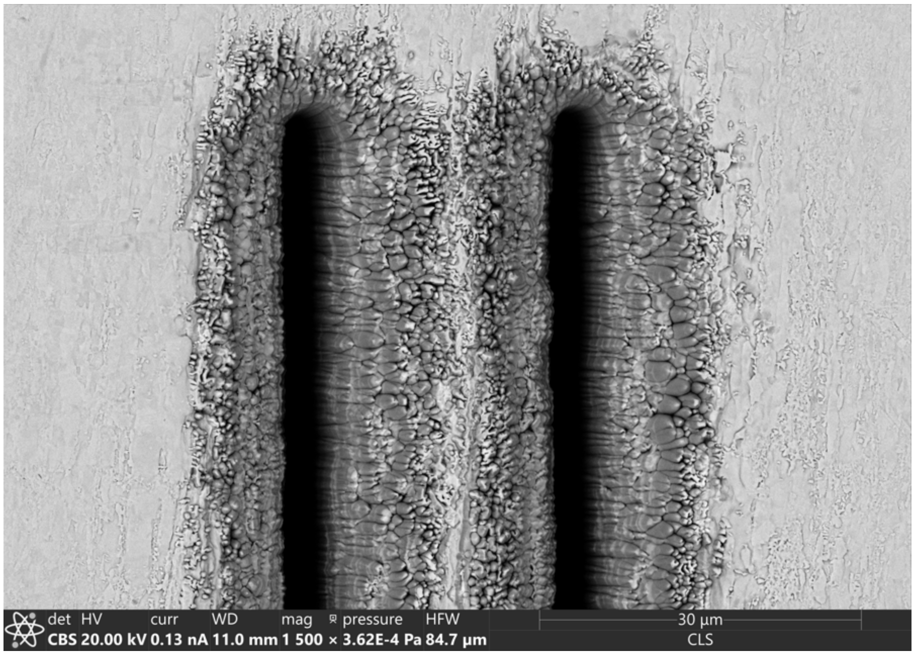


Fig. S2: Displayed is the SEM image taken for the 20 µm double slit.

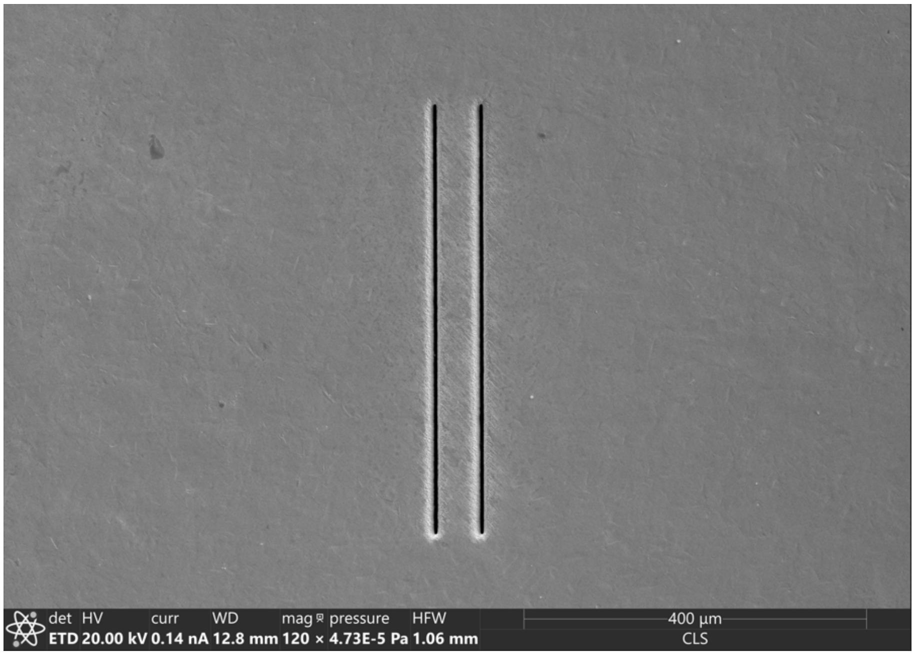


Fig. S3: Displayed is the SEM image taken for the 50 µm double slit.

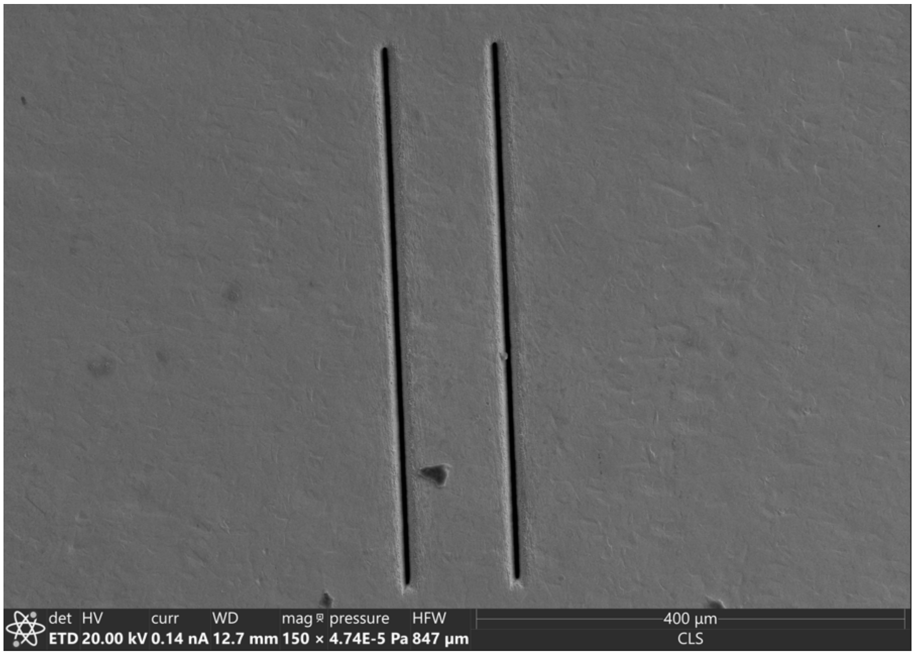


Fig. S4: Displayed is the SEM image taken for the 100 µm double slit.

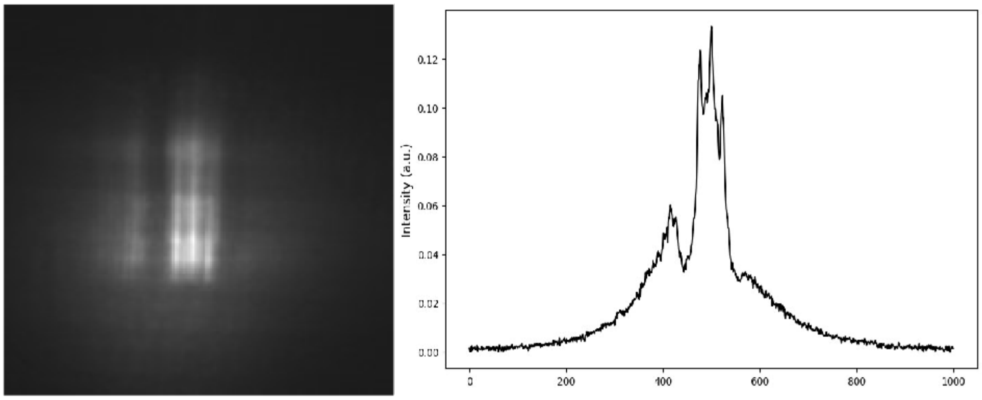


Fig. S5: Displayed are the interference fringes observed at E=20keV as well as the associated intensity distribution. As described in the paper, a combination of transmission through the slits and sampling issues rendered this data set unviable for analysis.

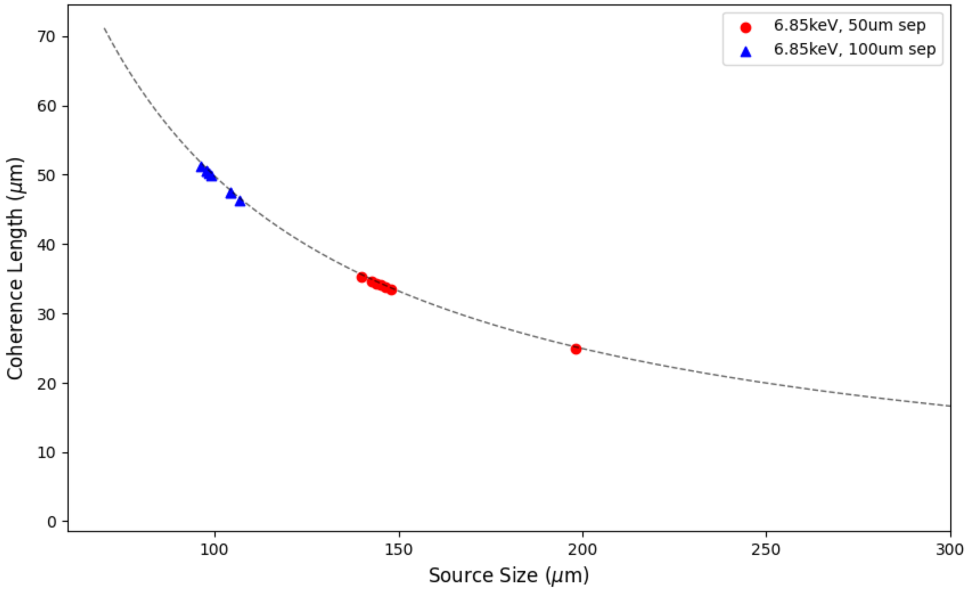


Fig. S6: Shown are the results for spatial coherence length measurements along the vertical component at E=6.85 keV. These values are up to double of what was see in the horizontal component. Due to the smaller vertical electron beam size, this result was expected. Plotted with the real data is the dashed line representing the theory curve. The circle markers represent the data taken with the 50 µm double slits while the triangle markers represent the data taken with 100 µm.

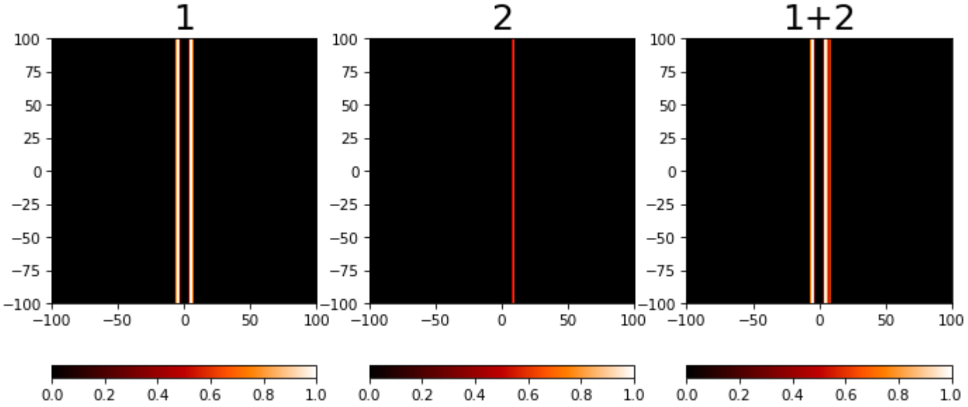


Fig. S7: Displayed is the process used to build the double slit mask for the asymmetric double slit simulation. The first subfigure represents an ideal pair of double slits, while the second subfigure contains a 1 µm slit that will be added to the double slit to produce the final asymmetric double slit.

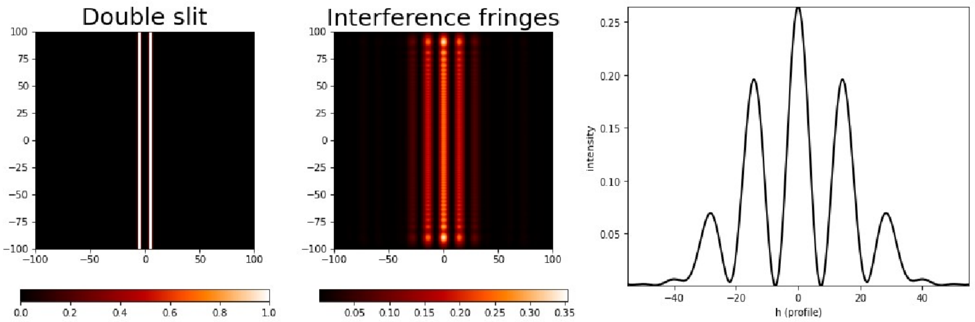


Fig. S8: Displayed are the simulation results for a double slit experiment in which the slits are of equal width. As expected, the interference fringes are symmetric.

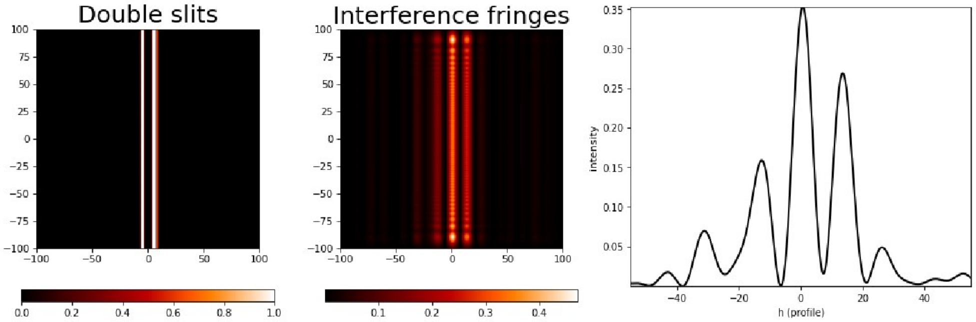


Fig. S9: Displayed are the simulation results for a double slit experiment in which the slits are of unequal width. A strong phase ramp is shown in the interference fringes.

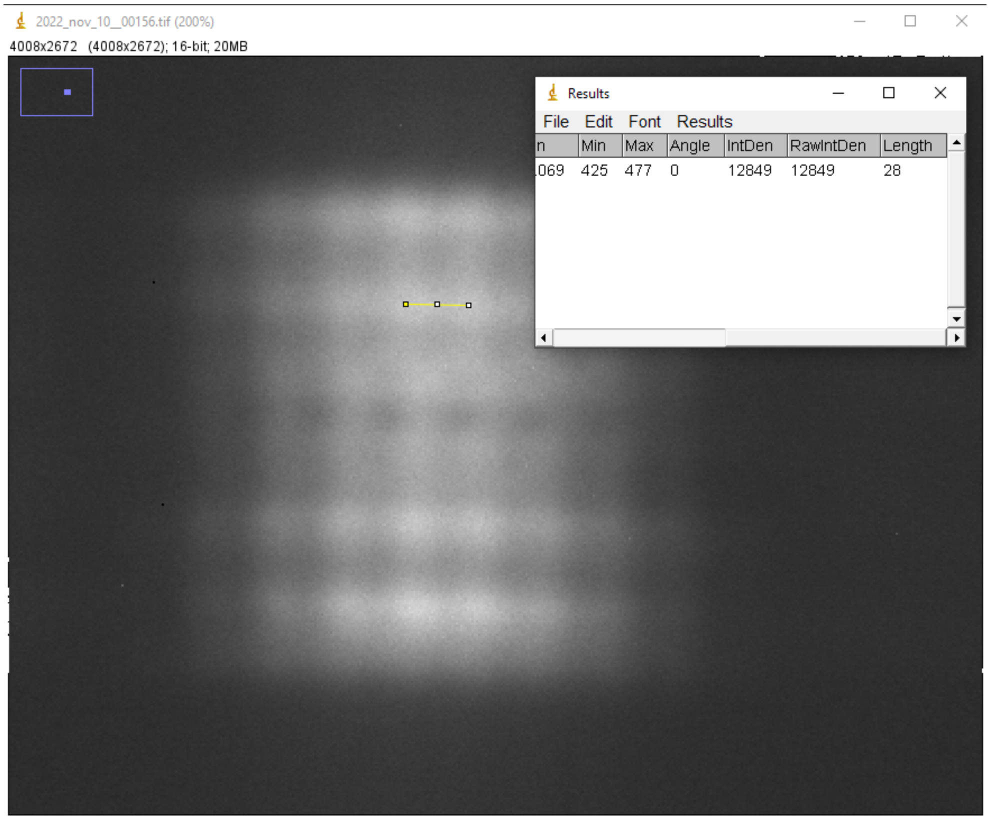


Fig. S10: Displayed is the direct measurement of interferometric fringe width from one of the images obtained during the experiment.

| Image Name | Slit Separation (µm) | Energy (keV) | Effective Pixel Size (µm) |
|---|---|---|---|
| Image156 | 11.612 | 6.75 | 3.39 |
| Image157 | 11.612 | 6.75 | 2.879 |
| Image159 | 11.612 | 6.75 | 2.996 |
| Image163 | 11.612 | 6.75 | 3.062 |
| Image179 | 20.909 | 6.75 | 2.929 |
| Image180 | 20.909 | 6.75 | 2.774 |
| Image181 | 20.909 | 6.75 | 3.101 |
| Image183 | 20.909 | 6.75 | 2.929 |
| Image72 | 11.612 | 7.5 | 3.164 |
| Image74 | 11.612 | 7.5 | 3.051 |
| Image75 | 11.612 | 7.5 | 3.051 |
| Image77 | 11.612 | 7.5 | 3.164 |
| Image79 | 11.612 | 7.5 | 2.946 |
| Image80 | 11.612 | 7.5 | 2.848 |
| Image83 | 11.612 | 7.5 | 3.051 |
| Image99 | 20.909 | 7.5 | 2.965 |
| Image101 | 20.909 | 7.5 | 3.163 |
| Image31 | 11.612 | 9.6 | 2.902 |
| Image33 | 11.612 | 9.6 | 3.034 |
| Image36 | 11.612 | 9.6 | 3.034 |
| Image40 | 11.612 | 9.6 | 2.902 |
| Image41 | 11.612 | 9.6 | 3.034 |
| Image42 | 11.612 | 9.6 | 3.178 |
| Image43 | 11.612 | 9.6 | 3.034 |
| Image44 | 11.612 | 9.6 | 2.902 |
| Image45 | 11.612 | 9.6 | 2.902 |
| Image57 | 20.909 | 9.6 | 2.648 |
| Image59 | 20.909 | 9.6 | 3.089 |
| Image60 | 20.909 | 9.6 | 2.851 |
| Image113 | 11.612 | 15 | 2.848 |
| Image116 | 11.612 | 15 | 3.051 |
| Image118 | 11.612 | 15 | 2.848 |
| Image119 | 11.612 | 15 | 3.051 |
| Image120 | 11.612 | 15 | 2.67 |
| pco4 | 51.685 | 6.85 | 0.808 |
| pco5 | 51.685 | 6.85 | 0.778 |
| pco6 | 51.685 | 6.85 | 0.751 |
| pco7 | 51.685 | 6.85 | 0.778 |
| pco8 | 51.685 | 6.85 | 0.725 |
| pco9 | 51.685 | 6.85 | 0.751 |
| pco10 | 51.685 | 6.85 | 0.841 |
| pco12 | 100.77 | 6.85 | 0.77 |
| pco13 | 100.77 | 6.85 | 0.719 |
| pco14 | 100.77 | 6.85 | 0.719 |
| pco15 | 100.77 | 6.85 | 0.674 |
| pco16 | 100.77 | 6.85 | 0.77 |
| pco17 | 100.77 | 6.85 | 0.719 |
| pco18 | 100.77 | 6.85 | 0.719 |



Table 2: Displayed are the measurements taken of the effective pixel size for both PCO detectors.

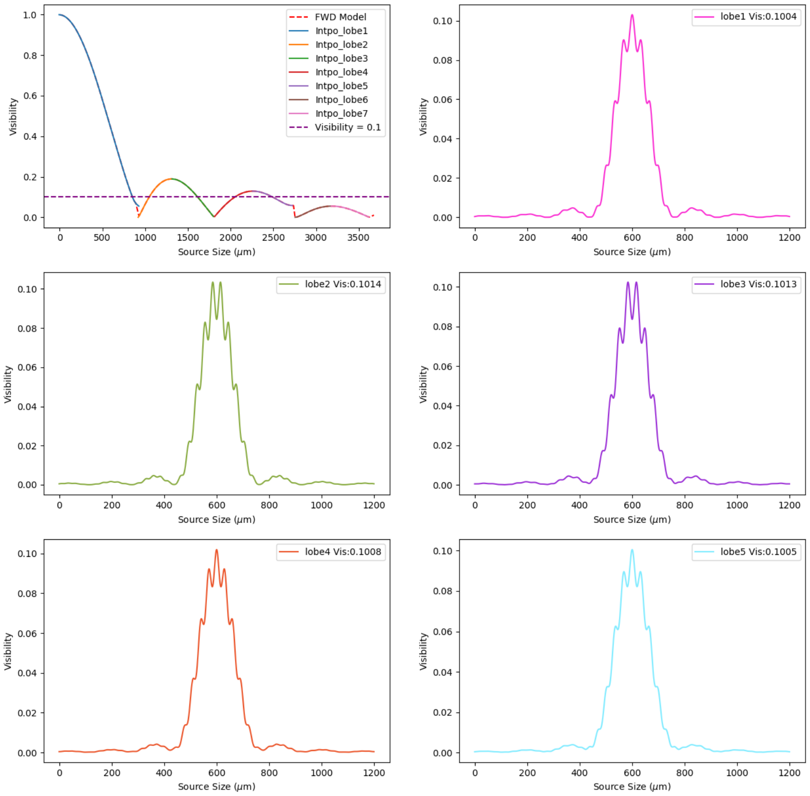


Fig. S11: Figure showing the inherent ambiguity of Visibility Vs Source Size curve. Below certain visibility value defined as maximum visibility before ambiguity (**MVBA**), the source size resulting in a given blurred intensity pattern is inherently ambiguous. One can clearly see this from the figure. The Visibility Vs Source Size curve is divided into 7 lobes where the resultant fringe patterns have same visibilities for widely varying source size values. It should be further noted that the MVBA can be further divided into MVBA by visibility and MVBA by form. Here we can see the MVBA by visibility between lobe1 to lobe5 and MVBA by form between lobe1 and lobe4,lobe5 as well as in lobe2 and lobe3.

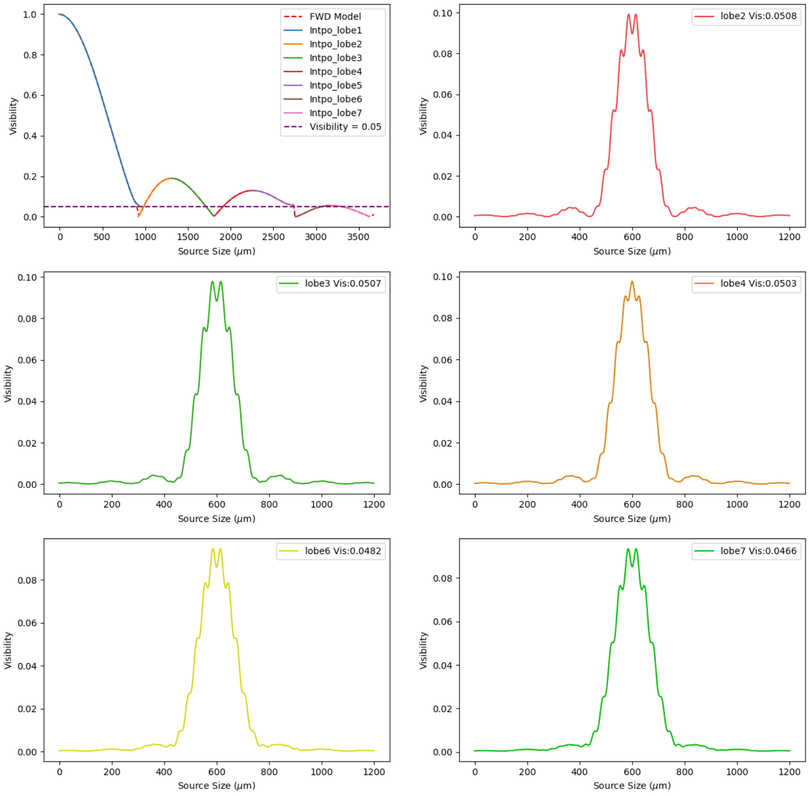


Fig. S12: Here we can see the MVBA by visibility between lobe2, lobe3, lobe4, lobe6 and lobe7 and MVBA by form between lobe2, lobe3 and lobe6, lobe7. For low enough visibilities like the one shown here, one can expect ambiguity through all the lobes both in terms of visibility and form.

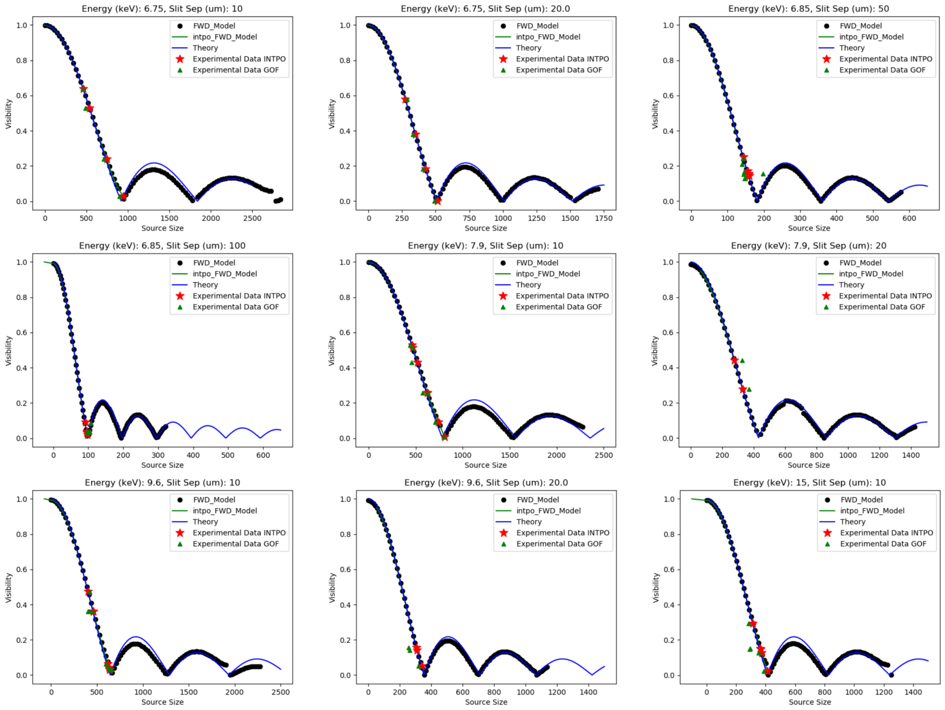


Fig. S13: Visibility vs Source size curves obtained through forward model, interpolated forward model and theory curves. The experimentally observed visibility values and their source size counter parts obtained from goodness of fit (GOF) and interpolation (INTPO) method are also shown. The subplots are compartmentalized by energy and slit separation.
